# Supplementary material for: Exploiting Energy Accumulation Against Co-channel Interference in Wireless Energy Harvesting MIMO Relaying
Source: arXiv:1609.09161 source file (2016-09-29)
Supplement: Supplementary file 1 [file Appendix_A.tex]

\subsection{Proof of Lemma \ref{lemma:PDF}}\label{append:proof_lemma_PDF}
